# Supplementary material for: All centralising monoids with majority witnesses on a four-element set
Source: arXiv:2011.00338 ancillary file (2020-10-31)
Supplement: Supplementary file 1 [file short_description_of_files.pdf]

## Short overview of the ancillary files

**cpp/** A directory containing undocumented and untidy `c++`-source files of the routines that were used to compute the contexts. These are provided for the sake of verification or error spotting; however a warning is due: they are provided as is and come with no explanation of which functions have to be called in which order on which type of input to achieve a certain type of goal. Anyone who is really interested in these details has to do his own guesswork. At the moment the author does not feel in a position to provide a more useful version of the code. Also all (intermediate) output files that sometimes (perhaps after some massaging) need to be reused as inputs for other tasks have not been included in order to avoid too much clutter.

This directory contains the following files:

**commutationMS.cpp** The main file to compute the contexts. Often standard output has to be redirected into a file to save the computed results.

**conjugate\_classes\_of\_majority\_ops.cpp** A file to split up the 392 majority operations into 90 conjugacy classes.

**maximal\_majority\_monoids.cpp** A file to compute which centralising monoids are maximal under inclusion.

**test\_uglies.cpp** This is a file to be included into **commutationMS.cpp** to deal with attributes that are unary operations with a three-element image (cf. Subsection 4.3 of the paper).

**conjugacy\_classes\_of\_392\_majority\_operations\_of\_K2.txt** The 392 majority operations that occur as objects of the context  $K''$  (see Table 5 in the paper) separated into 90 distinct conjugacy types (by the action of  $\text{Sym}(\{0, 1, 2, 3\})$ ).

**context\_K1.cxt** The context  $K'$  in BURMEISTER format<sup>1</sup>, see before Theorem 5.1 in the paper for a description.

---

<sup>1</sup>This is a very simple format for storing formal contexts using the following convention:

**context\_K2.cxt** The context  $\mathbb{K}''$  in BURMEISTER format, see before Theorem 5.1 in the paper for a description and cp. Tables 1 to 4 *ibid*.

**context\_K2\_extended.cxt** An extended version of the context  $\mathbb{K}''$  in BURMEISTER format. Instead of 167 attributes as in  $\mathbb{K}''$ , all 256 unary operations are used as attributes; the objects are identical to those of  $\mathbb{K}''$  (cf. Table 5 in the paper).

**context\_K3.cxt** The fully reduced and clarified context  $\mathbb{K}'''$  in BURMEISTER format, see before Theorem 5.1 in the paper for a description.

**list\_of\_147\_maximal\_monoids.txt** List of all 147 centralising monoids on  $\{0, 1, 2, 3\}$  with majority witnesses that are distinct from the full transformation monoid and maximal with respect to set inclusion among these (cf. Corollary 5.5 and Tables 8 and 9 in the paper).

**list\_of\_1715\_monoids.txt** List of all 1715 centralising monoids on the set  $\{0, 1, 2, 3\}$  having any set of majority operations as witnesses (cf. Corollary 5.2 in the paper).

**short\_description\_of\_files.pdf** This file.

**unary\_conjugation\_table.txt** A table showing the conjugation action of  $\text{Sym}(\{0, 1, 2, 3\})$  on all unary operations on the set  $\{0, 1, 2, 3\}$  via  $(s, f) \mapsto s \circ f \circ s^{-1}$ . Unary operations  $f: \{0, 1, 2, 3\} \rightarrow \{0, 1, 2, 3\}$  are represented as integers  $n = \sum_{j=0}^3 f(j)4^{3-j}$ .

---

line 1 = the letter ‘B’ (for Peter Burmeister), line 2 = blank, line 3 = number of objects (say  $m$ ), line 4 = number of attributes (say  $n$ ), line 5 = blank, lines 6...5 +  $m$  = labels for the objects (one per line), lines 6 +  $m$ ...5 +  $m$  +  $n$  = labels for the attributes (one per line), lines 6 +  $m$  +  $n$ ...5 + 2 $m$  +  $n$  = the rows of the context (denoting incidence by ‘X’ and non-incidence by ‘.’ with no spaces or other separators in between the columns, that is, these lines represent the characteristic vectors of the object intents when . is identified with 0 and X with 1).
